# Supplementary material for: Incorporating Geo-Diverse Knowledge into Prompting for Increased Geographical Robustness in Object Recognition
Source: arXiv:2401.01482 source file (2024-03-29)
Supplement: Supplementary file 1 [file X_suppl.tex]

k\clearpage
\setcounter{page}{1}
\maketitlesupplementary

\section{Rationale}
\label{sec:rationale}
Having the supplementary compiled together with the main paper means that:
\begin{itemize}
\item The supplementary can back-reference sections of the main paper, for example, we can refer to \cref{sec:intro};
\item The main paper can forward reference sub-sections within the supplementary explicitly (e.g. referring to a particular experiment); 
\item When submitted to arXiv, the supplementary will already included at the end of the paper.
\end{itemize}
To split the supplementary pages from the main paper, you can use \href{https://support.apple.com/en-ca/guide/preview/prvw11793/mac#:~:text=Delete%20a%20page%20from%20a,or%20choose%20Edit%20%3E%20Delete).}{Preview (on macOS)}, \href{https://www.adobe.com/acrobat/how-to/delete-pages-from-pdf.html#:~:text=Choose%20%E2%80%9CTools%E2%80%9D%20%3E%20%E2%80%9COrganize,or%20pages%20from%20the%20file.}{Adobe Acrobat} (on all OSs), as well as \href{https://superuser.com/questions/517986/is-it-possible-to-delete-some-pages-of-a-pdf-document}{command line tools}.

\begin{table}
    \begin{center}
    \begin{tabular}{c|c|c|ccc|}
    \hline
     Countries  &  LLM &  In   & Source & Target  \\
    
  in Ensemble &  Desc &  Country  & Acc &  Acc  \\
    
    \hline\hline
    Source & & \checkmark &  72.5 &  62.8 \\
    \hline
    Target & & \checkmark &  71.8 &  63.5  \\
    \hline
    All & & \checkmark &  72.8 &  63.2 \\
    \hline\hline
    Source & \checkmark &  &  73.0 &  63.4  \\
    \hline
    Target & \checkmark &  &  73.2 &  63.2  \\
    \hline
    All & \checkmark &  &  72.3 & 63.4 \\
    \hline
    \hline
    Source & \checkmark & \checkmark & 73.5  &  63.1  \\
    \hline
    Target & \checkmark & \checkmark & \textbf{73.6} &  \textbf{64.0}  \\
    \hline
    All & \checkmark & \checkmark & 72.6 &  63.8 \\
    \hline
    \end{tabular}
    \end{center}
    \caption{Comparing regularization results using different country ensemble sets and prompt formats. ViT }
    \label{tabel:all_src_tgt_reg}
\end{table}
