# Supplementary material for: Incorporating Geo-Diverse Knowledge into Prompting for Increased Geographical Robustness in Object Recognition
Source: arXiv:2401.01482 source file (2024-03-29)
Supplement: Supplementary file 3 [file supp_top5_bottom5_histogram_geonet.tex]

\begin{figure}[!tp]
    \centering
    \includegraphics[scale=0.5]  % Adjust the scale as needed
    {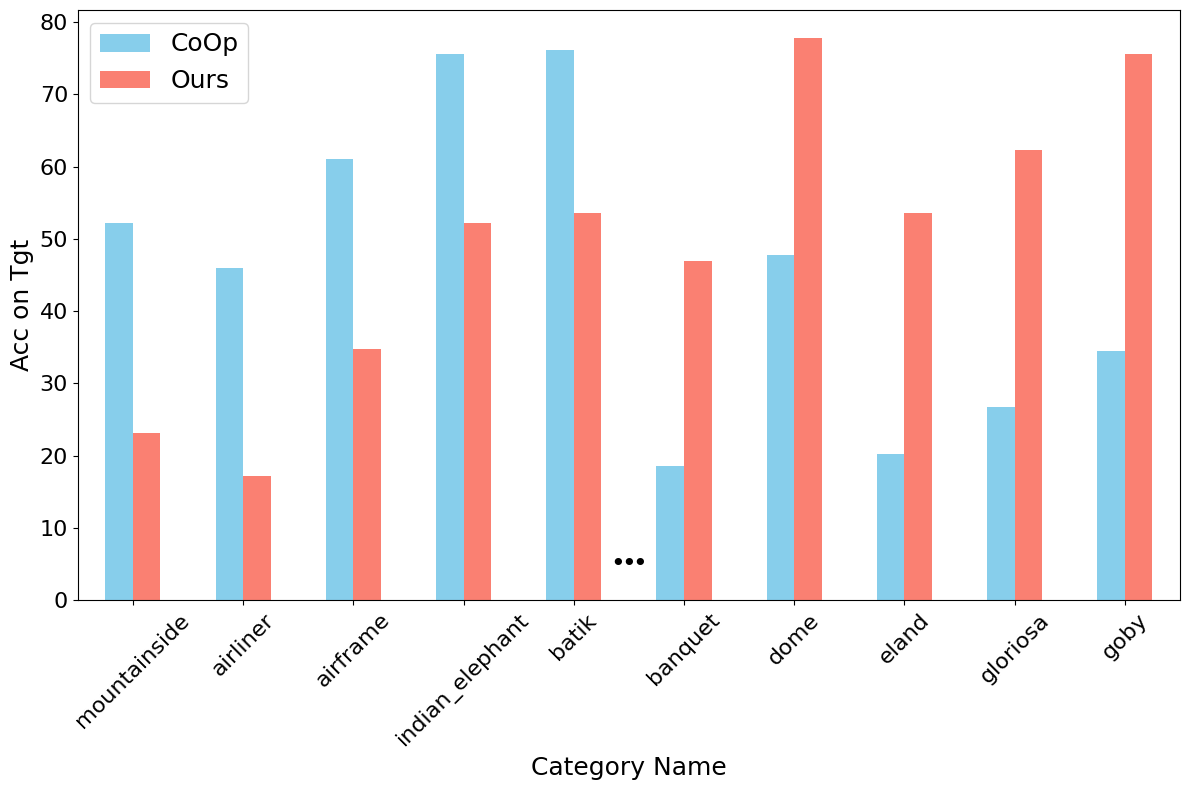}
    \vspace{-3mm}
    \caption{\textbf{Class-wise comparison of Ours vs. CoOp on GeoNet.} We sort the top 25 most frequent categories based on $\Delta = Acc(Ours) - Acc(CoOp)$ and show the bottom 5 and top 5 categories. Leveraging LLM descriptors can be most useful on objects that may have country-specific characteristics, while it may hurt the performance on more generic objects such as \textit{airliner} as it produces fine-grained descriptors like \textit{having two engines} which may not be visible in the image.}
    \label{supp:top5_bottom5_geonet}
\end{figure
}
